# Supplementary material for: PIN: Positional Insert Unlocks Object Localisation Abilities in VLMs
Source: arXiv:2402.08657 source file (2024-02-13)
Supplement: Supplementary file 1 [file main_suppl.tex]

\begin{table*}[!ht]
\centering
\resizebox{\textwidth}{!}{%
\begin{tabular}{l ccccc | ccccc }
\toprule
\multirow{2}{*}{Method} &\multicolumn{1}{c}{} & \multicolumn{4}{c}{$\text{PVOC}_{\leq 3 \text{ Objects}}$ } & \multicolumn{4}{c}{$\text{COCO}_{\leq 3 \text{ Objects}}$ } \\
% \cline{2-11}
& zero-shot &mIoU & $\text{mIoU}_M$ & $\text{mIoU}_L$ & $\text{mAP}_L$ & mIoU & $\text{mIoU}_M$ &  $\text{mIoU}_L$ & $\text{mAP}_L$  \\
\midrule
% random bbox generator& \cmark & 0.05 & 0.04 & 0.07 & 2.0 & 0.06 & 0.04 & 0.07 & 1.4  \\
% random bbox old &\cmark& 0.09 $\pm$ 0.06 & 0.03 $\pm $0.02 & 0.14$\pm$ 0.10& 4.9$\pm$ 1.3 & 0.07$\pm$ 0.06 & 0.04 $\pm$ 0.3 & 0.13 $\pm$ 0.12 & 4.1 $\pm $2.1 \\
random bbox selector &\cmark& 0.16 $\pm$ 0.01 & 0.09$\pm$0.01 & 0.23$\pm$ 0.02& 4.9 $\pm$ 1.3 & 0.09 $\pm$ 0.03 & 0.06 $\pm$ 0.1 & 0.16 $\pm$ 0.07 & 4.1 $\pm$ 2.1 \\
\midrule
OpenFlamingo~\cite{openflamingo_awadalla} & & & & & & & & &  \\
\hspace{3mm} raw  & \cmark & 0 & 0 & 0 & 0 & 0 & 0 & 0 & 0  \\
\hspace{4mm} + 2 context & (\cmark) & 0.16 $\pm $0.03 & 0.06 $\pm$ 0.02& 0.25 $\pm$ 0.05 & 6.3 $\pm$ 0.6  & 0.11 $\pm$ 0.03 & 0.06 $\pm$ 0.02 & 0.19 $\pm$ 0.05 & 5.1 $\pm $0.4 \\
\hspace{4mm} + 3 context & (\cmark) & 0.19 $\pm$ 0.02 & 0.07 $\pm$ 0.02& 0.28 $\pm$ 0.02& 10.6 $\pm$ 2.2 &0.06 $\pm$ 0.06 & 0.04 $\pm$ 0.04 & 0.11 $\pm$ 0.10 & 2.0 $\pm$ 1.7 \\
\hspace{4mm} + 5 context & (\cmark) & 0.09 $\pm$ 0.07 & 0.03 $\pm$ 0.02 & 0.14 $\pm$ 0.10& 5.0 $\pm$ 3.8 & 0.07 $\pm$ 0.06& 0.04 $\pm$ 0.04 & 0.13 $\pm$ 0.12 & 2.3 $\pm$  2.6\\
\hspace{4mm} + 10 context & (\cmark) & 0.13 $\pm$ 0.03 & 0.04 $\pm$ 0.02 & 0.21 $\pm$ 0.04& 7.1 $\pm$ 1.2 & 0.02 $\pm$ 0.01& 0.01 $\pm$ 0.01 & 0.04 $\pm$ 0.03& 0.7 $\pm$ 0.3 \\
\hspace{4mm} + PIN & \cmark &\B 0.45 &\B 0.27 &\B 0.62 &\B 21.9 & \B 0.35 &\B 0.26 & \B 0.59 & \B 20.7 \\

% Add more rows as needed
% \midrule
% \textcolor{lightgray}{Faster RCNN~\cite{faster_rcnn}} & \textcolor{lightgray}{\xmark} & \textcolor{lightgray}{--}& \textcolor{lightgray}{--} & \textcolor{lightgray}{--} & \textcolor{lightgray}{$40.3 ^\star$} & \textcolor{lightgray}{--} & \textcolor{lightgray}{--} & \textcolor{lightgray}{--}  & \textcolor{lightgray}{$73.2 ^\star$} \\
% \textcolor{lightgray}{DETR~\cite{detr}} & \textcolor{lightgray}{\xmark} & \textcolor{lightgray}{--} & \textcolor{lightgray}{--} & \textcolor{lightgray}{--} & \textcolor{lightgray}{$43.3 ^\star$} & \textcolor{lightgray}{--} & \textcolor{lightgray}{--} & \textcolor{lightgray}{--} & \textcolor{lightgray}{--} \\

\bottomrule

\end{tabular}
}
\caption{Comparison on object localisation on a subset of PVOC~\cite{pvoc} and COCO~\cite{coco} with maximal 3 objects per image, yielding 3,582 and 2,062 test images respectively. We strongly improve on the OpenFlamingo~\cite{openflamingo_awadalla} in-context learning baseline. Note, that PIN does not rely on context images thus no standard deviation is reported.
We corrected the IoU results for the random bbox selector due to a copy mistake resulting in only minor changes.
}
\label{tab:method_comparison_suppl}
\vspace{-0.3cm}
\end{table*}
